# Supplementary material for: Flash Cache: Reducing Bias in Radiance Cache Based Inverse Rendering
Source: arXiv:2409.05867 source file (2024-09-09)
Supplement: Supplementary file 1 [file supptab1_smoothness.tex]

\begin{table*}[t]
%\begin{SCtable}[75]
\centering
\caption{
\textbf{Smoothness Ablations}
}
\vspace{-0.1in}
\begin{tabular}{l c@{\,\,\,\,}c@{\,\,\,\,}c}
    \toprule
    Method & NVS PSNR$\uparrow$ & Albedo PSNR$\uparrow$ & MAE$\downarrow$ \\ \hline

    \phantom{(a)} Ours & 34.915 & 30.345 & 3.355  \\
    \bottomrule
\end{tabular}
\label{tab:smoothness}
%\end{SCtable}
\end{table*}
